# Supplementary material for: Seifert surfaces in the 4-ball
Source: arXiv:2205.15283 ancillary file (2023-05-02)
Supplement: Supplementary file 1 [file additional_documentation.pdf]

# ADDITIONAL DOCUMENTATION FOR "SEIFERT SURFACES IN THE 4-BALL"

KYLE HAYDEN, SEUNGWON KIM, MAGGIE MILLER, JUNGHWAN PARK, AND ISAAC SUNDBERG

This document explains the computer calculations used in [HKM+22]. These calculations are carried out in SnapPy [CDGW]. Our discussion is adapted for running SnapPy inside of Sage [The19], which enables SnapPy's computations to be rigorously verified using interval arithmetic.

## A. Initial calculations in SnapPy and Seifert genus

The knot $K_T$ is shown below in Figure A, in the case that there are no additional twists in the ellipsis. We enter $K_T$ into SnapPy using the diagram's Dowker-Thistlethwaite code:

```
In:  K = Link('DT:[(-134,-44,-152,-62,96,182,120,-162,-72,-50,-126,
     110,4,92,-176,-34,132,226,-86,-204,-28,174,66,156,-138,-188,-102,
     -14,146,80,170,-112,-24,-130,-192,160,52,142,-98,-10,-116,-178,-222,
     202,30,-42,-150,-60,-168,184,122,16,-70,-136,-46,-154,6,94,180,-56,
     -164,-74,-140,48,108,2,32,68,158,20,-186,-100,-12,-118,82,172,64,
     -22,-128,-190,-104,54,144,78,-8, -114,-26,-90,40,-148,-58,-166,-76,
     124,18,106,-234,214,-230,-208,-36,-224, 84,228,-216,-196,-220,-232,
     198,-212,-206,38,-88,-200,-218,210,-194)]')
```

We calculate the Seifert genus via knot Floer homology (which can also be calculated directly using [Sza19]). For brevity, we suppress most of the output:

```
In:  K.knot_floer_homology()
Out: {..., 'seifert_genus': 3,...}
```

Further below we will describe a rigorously verified calculation of the symmetry group of $K_T$. As an (unverified) initial check, we may ask for the symmetry group directly in SnapPy:

```
In:  E = K.exterior()
In:  E.symmetry_group()
Out: 0
```

Now we consider the case that the ellipsis contains $n$ full twists, in which case we obtain a knot we refer to as $K_{T+n}$.

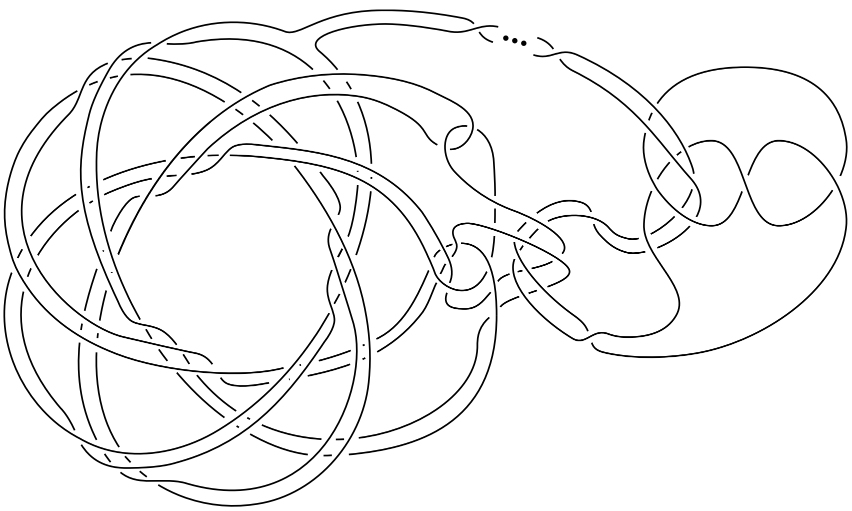

FIGURE A. When there are no twists in the ellipsis, this is $K_T$. When there are $n$ whole twists in the ellipsis, we obtain $K_{T+n}$.

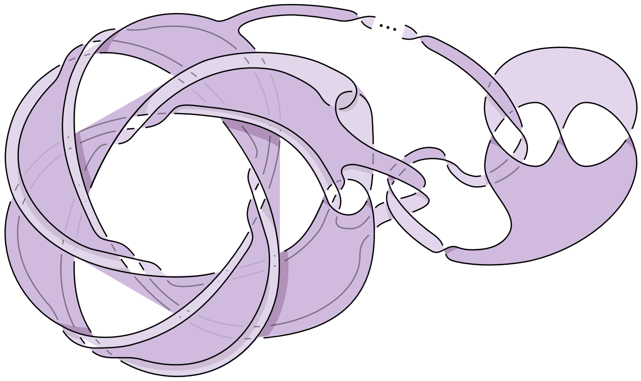

FIGURE B. A genus-3 Seifert surface for the knot $K_{T+n}$.

**Proposition A.1.** *For any integer $n$, the Seifert genus $g_3(K_{T+n})$ of $K_{T+n}$ is* 3.

*Proof.* The knot $K_{T+n}$ is a band sum of $\mathrm{Wh}(K)$ and a trefoil that bounds a genus-3 Seifert surface as in Figure B; adding full twists to the band corresponds to changing the integer $n$. The superadditivity of Seifert genus under band sums ([Gab87]) implies $g_3(K_{T+n}) \geq g_3(K) + g_3(T) = 2$. Moreover, equality holds only if $K_{T+n}$ has a minimal genus Seifert surface formed by summing minimal genus Seifert surfaces for $K$ and $T$ using the twisted band. If such a surface exists, then a surface of the same genus can be similarly constructed for any number of twists in the band, including $n = 0$. This contradicts our finding above that $g_3(K_T) = 3$. □

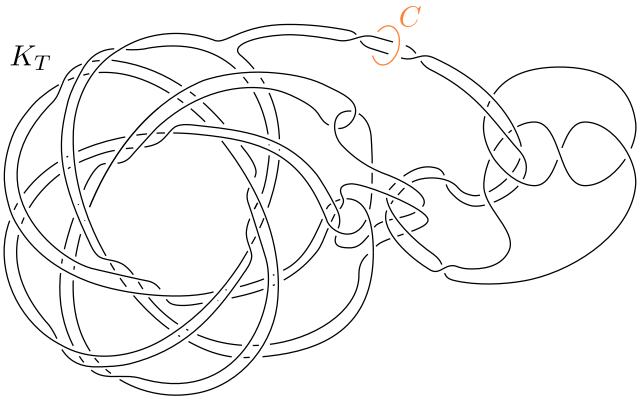


FIGURE C. The link $L = K_T \sqcup C$.

## B. VERIFYING THE SYMMETRY GROUP OF $K_{T+n}$

Let $L$ be the link shown in Figure C. This link has two components, labeled $K_T$ and $C$. The knot complement $S^3 \setminus K_T$ is obtained from the link complement $S^3 \setminus L$ by performing $\infty = 1/0$-filling on the unknotted component $C \subset L$. In Sage [The19], we import the SnapPy package and enter $L$ as a high-precision manifold using the diagram's Dowker-Thistlethwaite code:

```
In:  import snappy

In:  L = snappy.ManifoldHP('DT: [(-134,-44,-152,-62,96,182,120,-162,
    -72,-50,-126,110,4,92,-176,-34,132,228,-86,-206,-28,174,66,156,
    -138,-188,-102,-14,146,80,170,-112,-24,-130,-192,160,52,142,-98,
    -10,-116,-178,-224,204,30,-42,-150,-60,-168,184,122,16,-70,-136,
    -46,-154,6,94,180,-56,-164,-74,-140,48,108,2,32,68,158,20,-186,
    -100,-12,-118,82,172,64,-22,-128,-190,-104,54,144,78,-8,-114,-26,
    -90,40,-148,-58,-166,-76,124,18,106,-238,240,216,-232,-210,-36,
    -226,84,230,-218,-198,-222,-234,200,-214,-208,38,-88,-202,-220,
    212,-196,-242),(194,-236)]')
```

Our goal is to show that, for all $n \geq 0$, performing $(-1/n)$-framed Dehn filling along $C$ yields a hyperbolic 3-manifold with trivial isometry group. (This 3-manifold is homeomorphic to the complement of $K_{T+n}$.) As a preliminary step, we verify that the systole length of $S^3 \setminus L$ is at least 0.1428 by asking for the list of shortest geodesics:

```
In:   L.length_spectrum()

Out:  mult    length                   topology
      1       0.311...- 3.0236...*I    circle
      1       0.478...- 1.9665...*I    circle
```

It follows that the systole length is greater than 0.1428. Therefore, by [FPS19, Theorem 7.28], if the normalized length of the $-1/n$-filling slope is at least 10.1, then the filled manifold is hyperbolic and the core of the surgered solid torus is its unique shortest closed geodesic. In this case, it will follow that the isometry group after Dehn filling will be isomorphic to the isometry group of $S^3 \setminus L$ (which we will show below is trivial). To this end, we calculate the cusp areas:

```
 In:  L.cusp_areas()
Out:  [19.6907...18.8600...]
```

We are considering filling the second cusp, which we will also denote by $C$. The *normalized* length of a filling slope $\gamma$ on the cusp $C$ is given by $\text{Length}(\gamma)/\sqrt{\text{Area}(C)}$. To ensure a normalized length of at least 10.1, it suffices to consider slopes of unnormalized length at least 46:

$$\frac{\text{Length}(\gamma)}{\sqrt{\text{Area}(C)}} > \frac{46}{\sqrt{\text{Area}(C)}} \approx \frac{46}{\sqrt{18.6}} \approx 10.67 > 10.1$$

Next we ask for all slopes on the cusp $C$ up to unnormalized length 46 using the command `L.short_slopes(verified=True,length=46)`. SnapPy returns a list of slopes that include the $(-1/n)$-curves for $0 \leq n \leq 24$. For $n > 24$, it follows that the Dehn-filled manifold has the same isometry group as $S^3 \setminus L$, which we can show is trivial:

```
 In:  R = L.canonical_retriangulation(verified=True)
 In:  len(R.isomorphisms_to(R))
Out:  1
```

This shows that the isometry group consists of a single element, namely the identity. For the remaining slopes, we use a loop to verify that the filled manifold has trivial isometry group:

```
for n in range(0,25):
    L.dehn_fill((1,-n),1)
    Y = L.filled_triangulation()
    R = Y.canonical_retriangulation(verified=True)
    Y = R.with_hyperbolic_structure()
    Y.verify_hyperbolicity()
    len(R.isomorphisms_to(R))
```

For each value $n = 0, 1, ..., 24$, this prints a confirmation that the filled manifold is hyperbolic and that its isometry group is trivial.

## References

[CDGW] Marc Culler, Nathan M. Dunfield, Matthias Goerner, and Jeffrey R. Weeks. SnapPy, a computer program for studying the geometry and topology of 3-manifolds. `http://snappy.computop.org`.

[FPS19] David Futer, Jessica S. Purcell, and Saul Schleimer. Effective bilipschitz bounds on drilling and filling. *Geom. Topol. (to appear)*, arxiv:1907.13502, 2019.

[Gab87] David Gabai. Genus is superadditive under band connected sum. *Topology*, 26(2):209–210, 1987.

[HKM+22] Kyle Hayden, Seungwon Kim, Maggie Miller, JungHwan Park, and Isaac Sundberg. Seifert surfaces in the 4-ball. *arXiv:2205.15283*, 2022.

[Sza19] Zoltán Szabó. Knot Floer homology calculator. Available at `https://web.math.princeton.edu/~szabo/HFKcalc.html`, 2019.

[The19] The Sage Developers. Sagemath, the Sage mathematics software system. Available at `https://www.sagemath.org`, 2019.

Department of Mathematics, Columbia University, New York, NY 10027 USA
*Email address*: `hayden@math.columbia.edu`

Center for Quantum Structures in Modules and Spaces, Seoul National University, Seoul 08826, Republic of Korea
*Email address*: `math751@gmail.com`

Department of Mathematics, Stanford University, Stanford, CA 94305 USA
*Email address*: `maggie.miller.math@gmail.com`

Department of Mathematical Sciences, KAIST, Daejeon 34141, Republic of Korea
*Email address*: `jungpark0817@kaist.ac.kr`

Department of Mathematics, Bryn Mawr College, Bryn Mawr, PA 19010 USA
*Email address*: `isaacsundbe@gmail.com`
